# Supplementary material for: Spatial Dependence of Polycyclic Aromatic Compounds Growth in Counterflow Flames
Source: arXiv:1801.00666 source file (2017-12-28)
Supplement: Supplementary file 1 [file supmat.pdf]

# Spatial Dependence of Polycyclic Aromatic Compounds Growth in Counterflow Flames: Supplemental Material - Computational

Qi Wang[a], Paolo Elvati[a], Doohyun Kim[a], K. Olof Johansson[b], Paul E. Schrader[b], Hope A. Michelsen[b], Kevin R. Wilson[c], Angela Violi[a,d,*]

[a] *Department of Mechanical Engineering, University of Michigan, 2350 Hayward St., 2250 G.G. Brown, Ann Arbor, MI 48109-2125, United States*
[b] *Combustion Research Facility, Sandia National Laboratories, Livermore, CA 94550, United States*
[c] *Chemical Sciences Division, Lawrence Berkeley National Laboratory, Berkeley, CA 94720, United States*
[d] *Departments of Chemical Engineering, Biomedical Engineering, Macromolecular Science and Engineering, Biophysics Program, University of Michigan, Ann Arbor, MI, United States*

## 1. SNapS2 kinetic mechanism

The SNapS2 kinetic mechanism currently includes 288 generic reactions, grouped in five broad categories: carbon-hydrogen (C−H), carbon-carbon (C−C), oxygen-hydrogen (O−H), oxygen-carbon (O−C), and isomerizations. There are also a small number of uncategorized reactions, mainly to bridge reactions that would go in different categories, such as the transformation between five- and six-membered rings.

All reactions are fully reversible and thermodynamically consistent. The reverse reaction rates are calculated using the thermodynamics data from NASA-format polynomials. The NASA polynomial for one molecule has

*Corresponding author:
*Email address:* avioli@umich.edu (Angela Violi)

*Preprint submitted to Proceedings of the Combustion Institute* *December 21, 2017*

14 coefficients: the first 7 are for high temperature region (important for combustion) and the last 7 are for low temperature range. The enthalpy ($H_T^\circ$) and entropy ($S_T^\circ$) at a specific temperature can be calculated according to:

$$\frac{H_T^\circ}{RT} = a_1 + \frac{a_2}{2}T + \frac{a_3}{3}T^2 + \frac{a_4}{4}T^3 + \frac{a_5}{5}T^4 + \frac{a_6}{T} \tag{S1}$$

$$\frac{S_T^\circ}{R} = a_1 \cdot ln(T) + a_2 T + \frac{a_3}{2}T^2 + \frac{a_4}{3}T^3 + \frac{a_5}{4}T^4 + a_7 \tag{S2}$$

where, $R = 8.314 J/mol \cdot K$ is the universal gas constant, $T$ is the temperature, $a_1$ through $a_7$ are the 7 coefficients in NASA-format polynomial.

Then the following equations are used to compute the reverse reaction rates ($k_{reverse}$), and then fitted into extended Arrhenius form.

$$\Delta_r G_T^\circ = -RT \cdot ln(K) = \Delta_r H_T^\circ - T\Delta_r S_T^\circ \tag{S3}$$

$$k_{reverse} = \frac{k_{forward}}{K} \tag{S4}$$

### *1.1. C-H bond reactions*

This group includes all the reactions that result in a net formation or disruption on the tracked molecule of a C−H bond. For the abstractions we considered different gas-phase species, namely H, OH, O, $HO_2$, $O_2$, $CH_3$, $C_2H_3$, and $C_6H_5$. This category is further divided into three subclasses:

*Six-membered aromatic rings.* Hydrogen abstraction or C−H bond breaking from six-membered aromatic rings (single or condensed), with different substitutes.

*Five-membered aromatic rings.* Includes reactions from single (cyclopentadienyl radical) and condensed five-membered rings.

*Aliphatic carbons.* This is the largest subgroup as includes reactions in $\alpha$, $\beta$, and $\gamma$ to a variety of groups, *e.g.*, double and triple bonds, aromatic and aliphatic rings.

### *1.2. C-C bond reactions*

This group includes all the reactions that result in a net formation or disruption on the tracked molecule of a C−C bond. This category is further divided into two subclasses:

*Fragment addition/removal.* Fragment addition can happen with methylene ($CH_2$), methyl radical ($CH_3$), acetylene ($C_2H_2$), vinyl ($C_2H_3$), ethylene ($C_2H_4$), propargyl ($C_3H_3$), propene ($C_3H_6$), 1,2-butadiene ($C_4H_6$), phenyl ($C_6H_5$), and benzene ($C_6H_6$).

*Ring formation/opening.* This subcategory includes HACA ring closure, Diels-Alder reaction, ring closures with propargyl, cyclopentadienyl radical to six-membered ring, bay-site closure for both five- and six-membered rings.

### *1.3. O-H bond reactions*

This group includes all the reactions that result in a net formation or disruption on the tracked molecule of a O−H bond. For the abstractions we considered different gas-phase species, namely H, OH, O, $HO_2$, $O_2$, $CH_3$, $C_2H_3$, and $C_6H_5$. This category is further divided into two subclasses depending on the location (aliphatic or aromatic) of the hydroxy group, again with distinctions between six-membered and five-membered aromatic rings.

### *1.4. O-C bond reactions*

Oxygen can be added from the following gas-phase species: O, OH, $O_2$, and $HO_2$. Oxygenated groups can react with $C_2H_2$, $CH_3$, $C_6H_5$, and $C_6H_6$. This category is further divided into three subclasses:

*Aromatic.* Includes formation/disruption of bonds between oxygen and a carbon atom in an aromatic ring.

*Aliphatic.* Includes formation/disruption of bonds between oxygen and aliphatic carbons (in a chain or a rings).

*Ring closures.* Ring opening/closure of heteroaromatic rings, *e.g.*, furan rings.

### *1.5. Isomerizations*

Is composed by hydrogen transfer reactions. These reactions are distinguished depending on the type of both the starting and ending atom involved (*i.e.*, oxygen,aliphatic or aromatic carbon, )

## 2. Additional CFD data

The mole fraction contours of the gas-phase species OH, $C_2H_2$, $C_3H_3$, and $C_6H_6$ from the snapshot of the center plane of the 3D CFD simulation have been plotted in the Fig. S1.

The OH mole fraction peaked early leaning to the oxidizer side. As streamline approaching stagnation plane around a DFFO of 5 mm, OH mole fraction decreases very fast. The same is true for most oxygen-containing gas-phase species, *e.g.*, O and $O_2$.

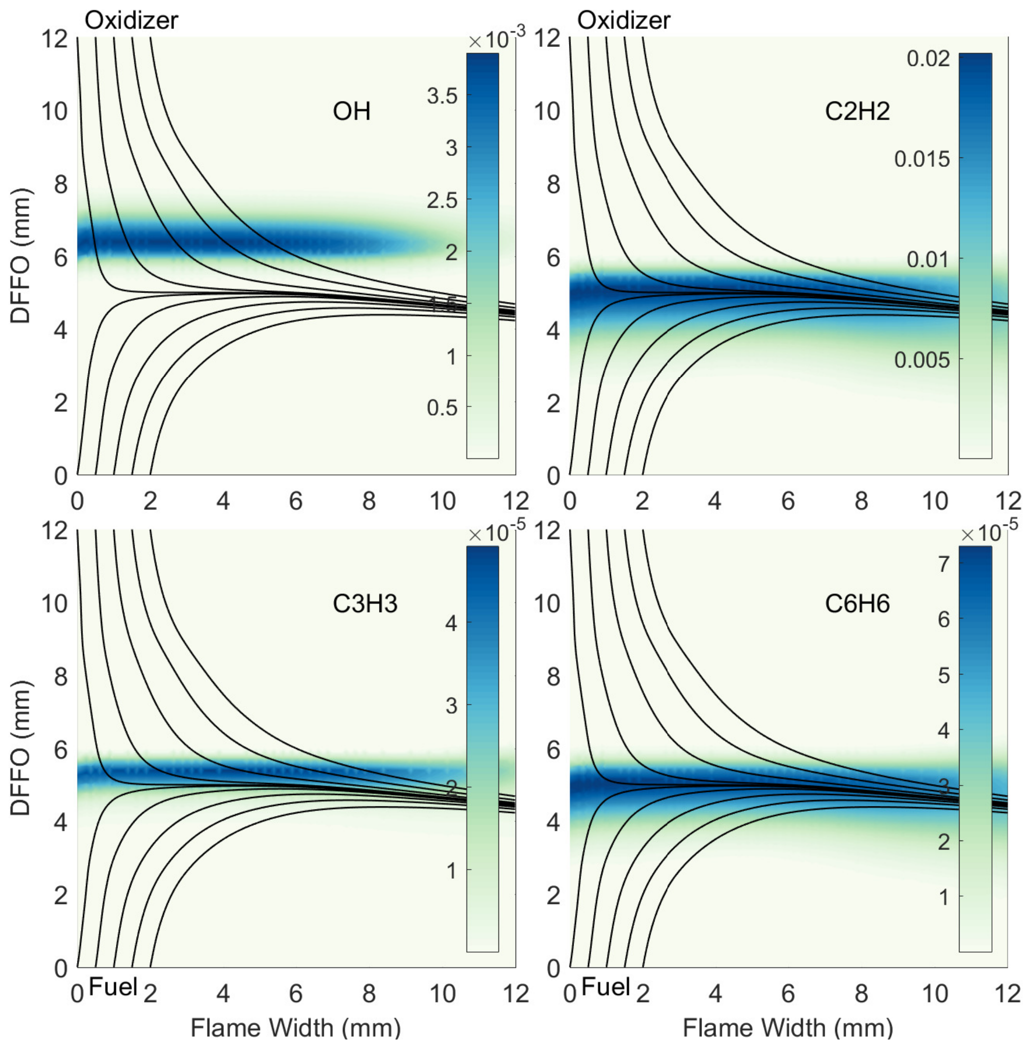


Fig. S1: Gas-phase species mole fraction contour for OH, $C_2H_2$, $C_3H_3$, and $C_6H_6$, from snapshot of the central plane of the CFD simulation. Black lines represents flow streamlines.

Both $C_2H_2$ and $C_6H_6$ mole fractions peak near stagnation plane along the streamlines, which is also a high-temperature region. Thus, as streamlines flowing through this region, HACA would dominate the molecular growth because of high temperature and $C_2H_2$ concentration. And since the oxygen-containing gas-phase species concentration is low at this region (*e.g.*, OH), pure hydrocarbons are mostly expected to be formed here, as observed in the SNapS2 simulation results.

## 3. Probe size analysis

Whereas the vertical sampling resolution (along centerline) is relatively high and enables the VUV-AMS experiments to resolve sub-mm vertical profiles, the horizontal width of the probe volume is uncertain. Thus, we performed a probe size analysis for the sampling width, by varying the probe area used to generate mass spectra from the SNapS2 simulations (see light gray region extending from the black dot in Fig. 1). We assumed that the section of the probe volume lying in the plane of Fig. 1 (of the paper) could be described by a half-ellipse with a semi minor axis of 0.25 mm. The semi major axes of the ellipse, *i.e.*, the sampling width, was varied between 0.5 and 2.5 mm. See the Fig. S2.

For widths less than 1.5 mm, the sampling area does not overlap with the simulated flow streamlines and therefore no spectra can be generated. However, for all sampling widths between 1.5 mm and 2.5 mm, the mass spectra shows the same mass peaks, with relative intensities slightly change. The paper Fig. 3b uses 2.5 mm as sampling width.

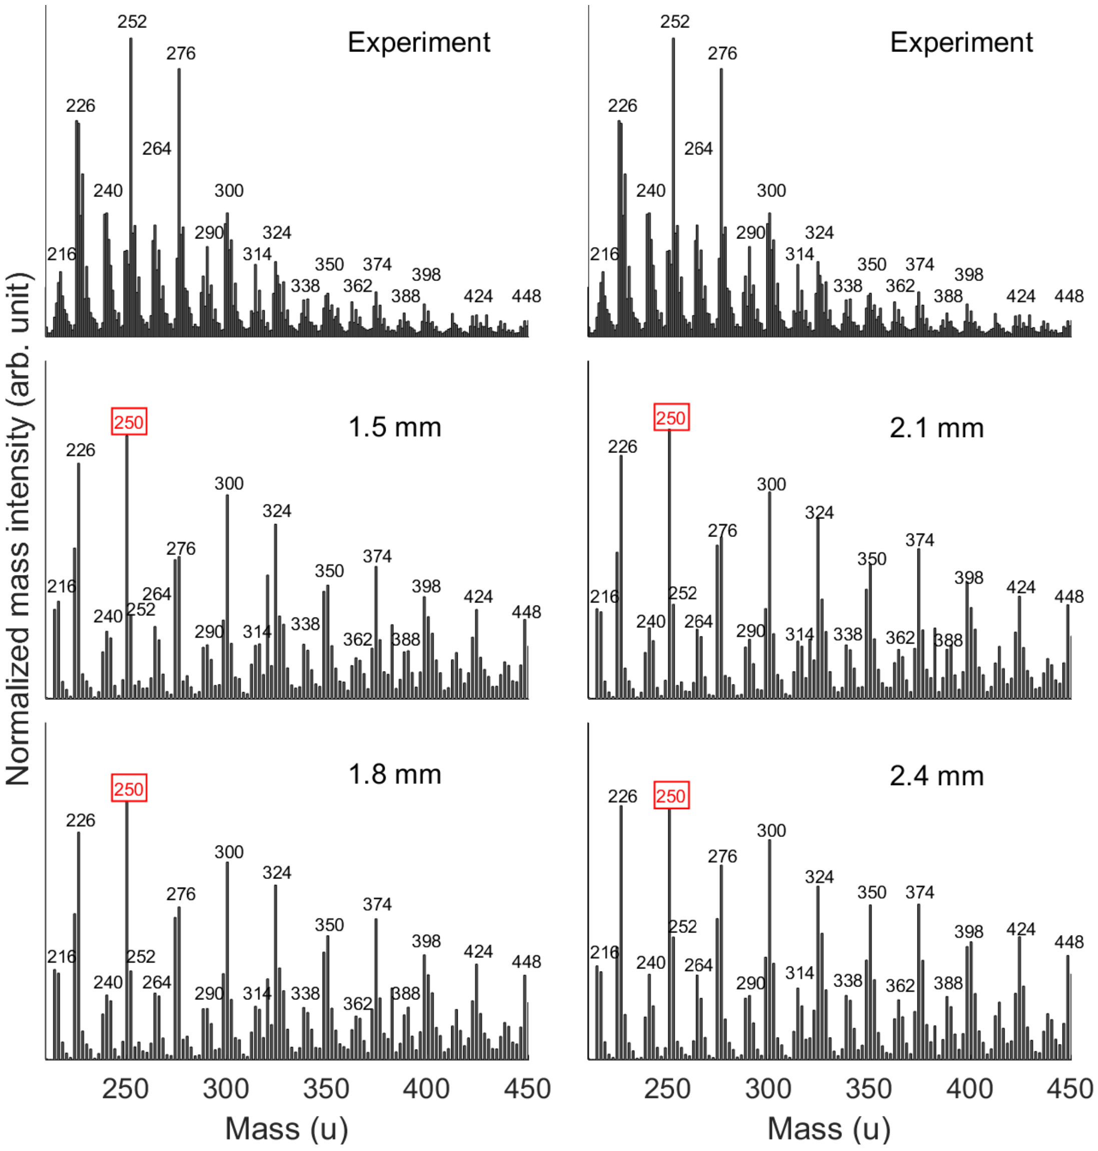


Fig. S2: SNapS2-generated spectra at DFFO = 5.0 mm using different sampling widths.

## 4. Error analysis

We conducted a detailed error analysis for the SNapS2-generated mass spectra shown in paper Fig. 3 and Fig. 5. The molecules generated by SNapS2 are weighed three times to generate the mass spectra: 1) particle life-time, 2) benzene seed concentration at the SNapS2 simulation starting points, and 3) the integral of the benzene concentration in the sampling area for one streamline, if multiple streamlines were included. Thus, the equation used to estimate the error (with a 95% confidence interval) for the intensity of a given mass (m) is:

$$\epsilon_m = 1.96 \sum_j c_j \sum_i w_{ij} \left( \frac{p_{ij}(1 - p_{ij})}{n_{ij}} \right)^{\frac{1}{2}} \tag{S5}$$

with $w_{ij}$ and $c_j$ are defined as:

$$\begin{aligned} w_{ij} &= c_{ij}\tau_{ij}, \\ c_j &= \int_{t_1}^{t_2} c(t)dt \end{aligned}$$

where $j$ is the index of the streamline, $i$ the starting point in the streamline $j$, $c$ is the seed concentration, $p$ is the probability of the given mass, and $n$ is the sample size. $\tau$ is the molecule lifetime, $t_1$ and $t_2$ are start and end point of sampling for each streamline.

The percentage error plots Fig. 3a and Fig. 3b are corresponding to Fig. 3 and Fig. 5 in the paper. As shown in Fig. S3, as sampling number of the particles increases, the percentage error is much lower. Nevertheless, the largest error in the main paper is 3.5%, which is relatively small for comparison of the identified mass peaks and their intensities.

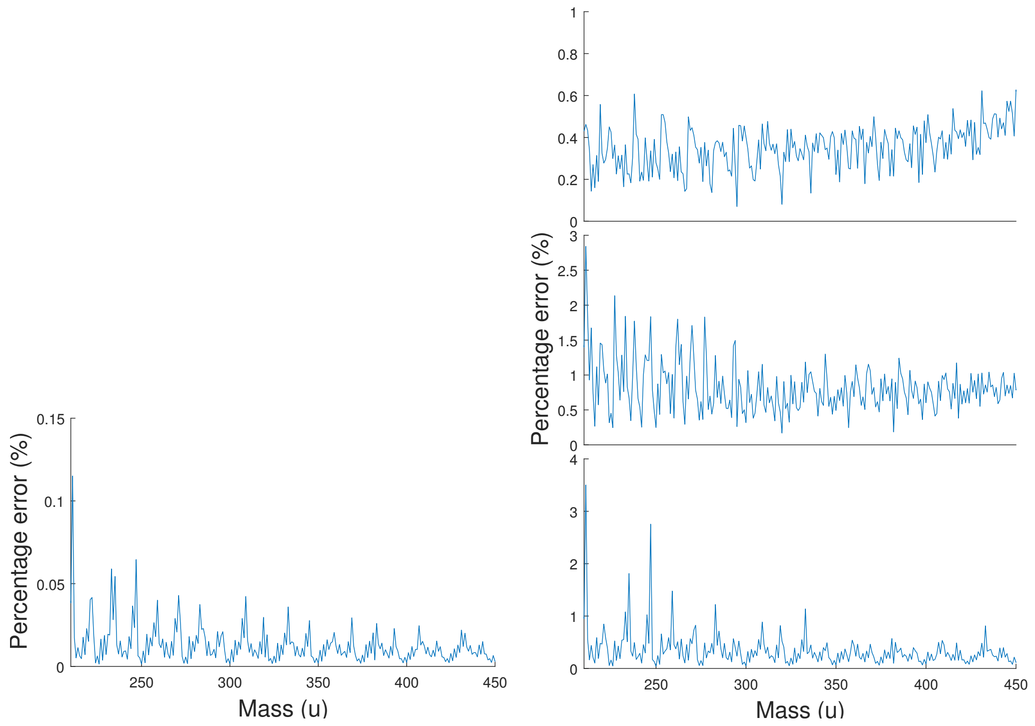


Fig. S3: Percentage error of SNapS2 mass spectra corresponding to Fig. 3 and Fig. 5 in the paper
